# Supplementary material for: OWL (Observe, Watch, Listen): Audiovisual Temporal Context for Localizing Actions in Egocentric Videos
Source: arXiv:2202.04947 source file (2022-10-26)
Supplement: Supplementary file 3 [file implementation.tex]

\section{Implementation details of HOMAGE experiments}
\label{sec:homage_impl}

First, we want to note that action annotations for HOMAGE are not decomposed into nouns and verbs as in EK100. Therefore, we adapt our model to directly provide  predictions for each action class. We train our model for 446 (out of 453) classes, as we removed some videos from the dataset due to the issues with their metadata.  
Similarly to EK100, we extract SlowFast visual \cite{feichtenhofer2019slowfast} and SlowFast auditory features \cite{kazakos2021slow} for the experiments on HOMAGE. The auditory features are extracted with  backbone pre-trained on VGG-Sound \cite{chen2020vggsound}, and the visual features with pre-trained backbones on EK100 \cite{damen2021rescaling}. We use features extracted at 1 FPS for both proposal generation and classification. For the proposal generator, we use a sliding window of size 160 and a stride of 80.
